# Supplementary material for: Modeling offensive content detection for TikTok
Source: arXiv:2408.16857 source file (2024-10-17)
Supplement: Supplementary file 1 [file 08appendix.tex]

%!TEX root = ../CLINtemplate.tex

\section{Scraping comments using Selenium}
 This section further explains how comments that belonged to each of these unique posts were automatically collected. As one needs an account to access the replies to a post, it is important te mention the fact that collecting these is against the TikTok TOS\footnote{\url{https://tiktok.com/legal/page/eea/terms-of-service}}.
 
Selenium is an open-source, cross-platform tool used for automating web browsers. Its primary function is to simulate user interactions such as clicking buttons, filling out forms, and navigating between pages, which makes it ideal for this use-case~\cite{ramya2017testing}.

A Python script\footnote{\url{https://github.com/kaspercools/tiktok-selenium-crawler}} was created for scraping the comments from posts collected using the steps described in the previous sections. Information related to these posts (e.g username and id of the post) was then used to build a URI path to a particular post. 
When navigating to a certain video post on TikTok, not all comments are immediately visible (Figure~\ref{fig:closed-comment-depth}). TikTok allows users to not only comment on a video, but also to react to one another, as shown in Figure~\ref{fig:single-comment-depth}. It is thus necessary to programmatically loop over these comments to check whether or not there are replies.
Furthermore, if a post has a lot of (nested)comments, the front-end might not immediately load all data at once due to virtualization, which is often used when handling larger datasets to optimize performance and enhance user experience on these types of platforms~\cite{kirichek2020implementation}.
For this reason, one needs to first scroll down the page so that all comments and their linked replies are loaded correctly, and accessible in the browser. This, in combination with other components that are sometimes loaded dynamically, causes one to have to wait while components are loaded. To give the browser an appropriate amount of time to load all of its components, implicit wait statements were added:
\begin{center}
    \begin{lstlisting}[language=Python, aboveskip=0pt, belowskip=0pt]
        driver.implicitly_wait(n)
    \end{lstlisting}
\end{center}

The previous statement allows the Document Object Model (DOM) to load its components~\cite{wood1998document}. The latter will simply poll for \(n\) time units until the DOM elements are ready.
As soon as all data is present, it is possible to collect comments. XPATH~\cite{clark1999xml} expressions are used to retrieve or invoke certain HTML components within the DOM, providing quick and easy access. Once the previous steps had been completed, the collected comments were saved in Javascript Object Notation (JSON), which allows the preservation of the relationships in regards to the comment tree structure~\cite{crockford2006rfc}.
\begin{figure}[h]
     \centering
     \begin{subfigure}[b]{0.48\textwidth}
         \centering
        \includegraphics[scale=0.4]{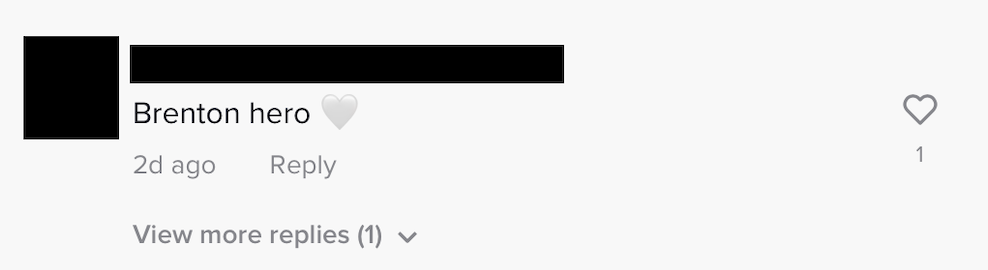}
        \caption{\label{fig:closed-comment-depth}in its initial state}
        
     \end{subfigure}
     \begin{subfigure}[b]{0.48\textwidth}
        \centering
        \includegraphics[scale=0.4]{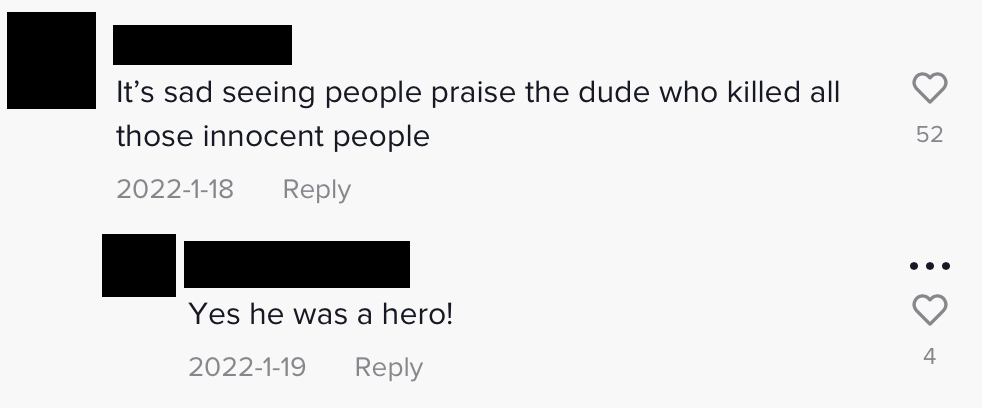}
        \caption{\label{fig:single-comment-depth}in open state}
     \end{subfigure}
        \caption{TikTok comment structure with a reply}
        \label{fig:tiktok-comment-structure}
\end{figure}

Lastly, before comments can be retrieved and read, one needs to be logged in. To accomplish this, remote debugging was enabled in the Chromium browser and subsequently, a valid TikTok session ID had to be available within that browser instance. That way, the Selenium script did not have to go through the process of logging into the account and was able to directly navigate to the desired TikTok post~\cite{sharma2012better}.

\clearpage
\section{Top 20 Data analysis charts}

\begin{figure}[h]
    \centering
		\includegraphics[scale=0.33]{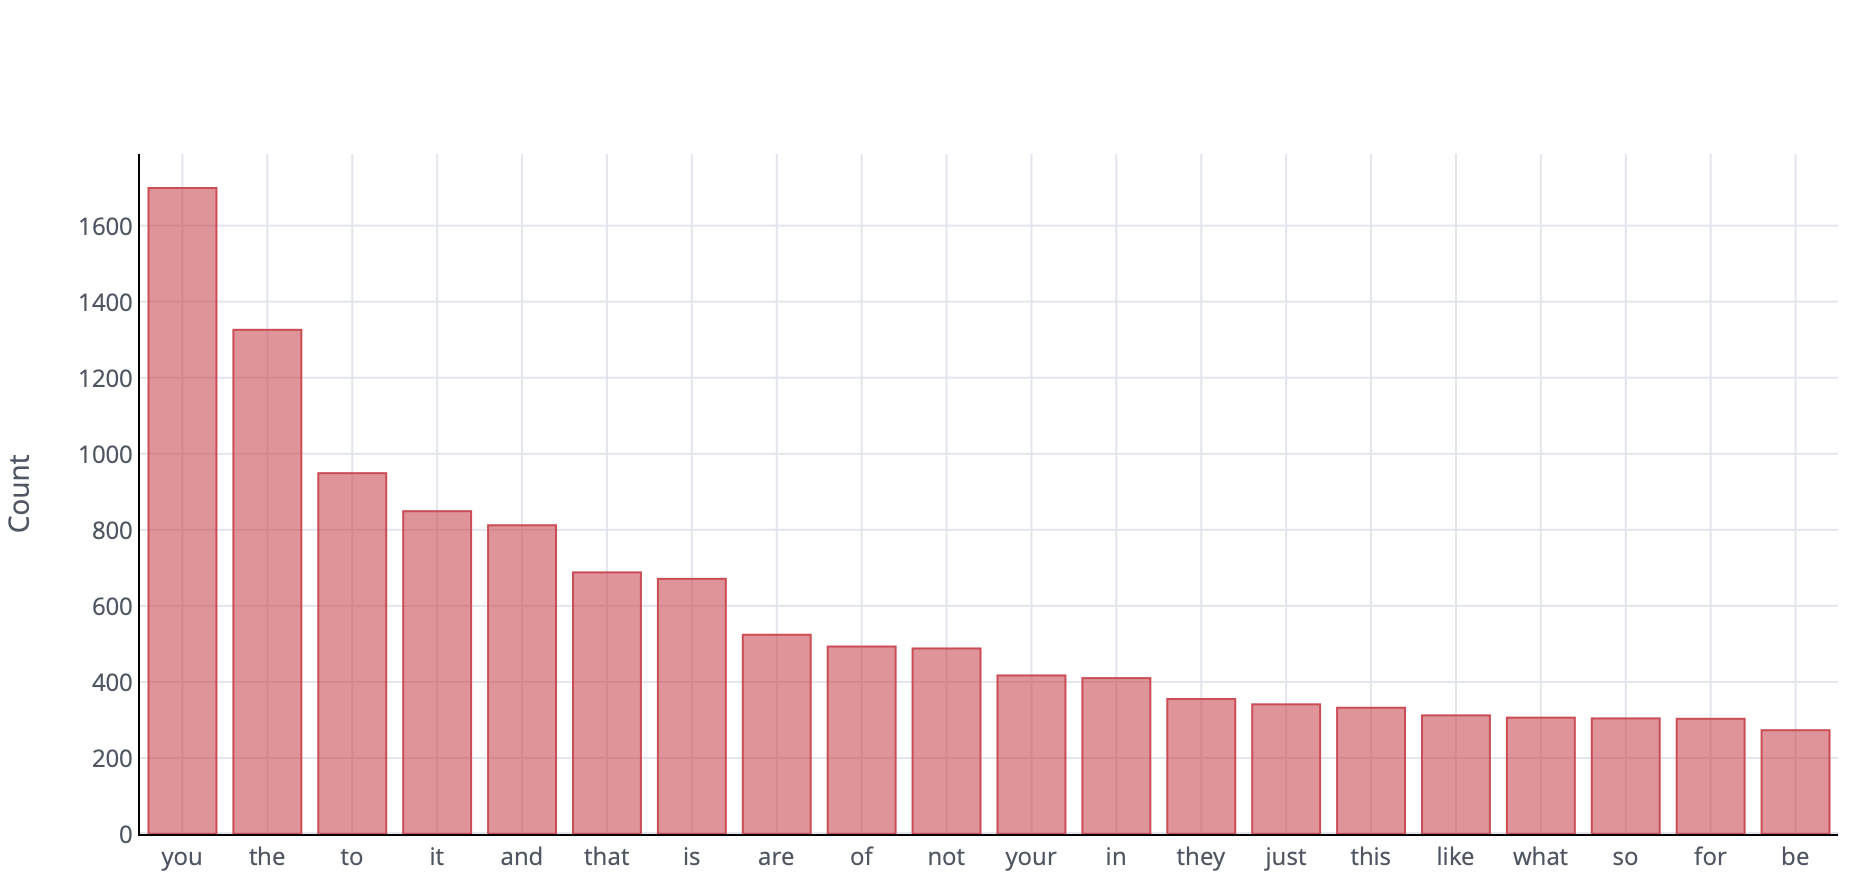}
		\caption{Top 20 words used for offensive comments before removing stop words}
		\label{fig:top20-before-removing-stopwords}
\end{figure}
\begin{figure}[h]
\centering
		\includegraphics[scale=0.33]{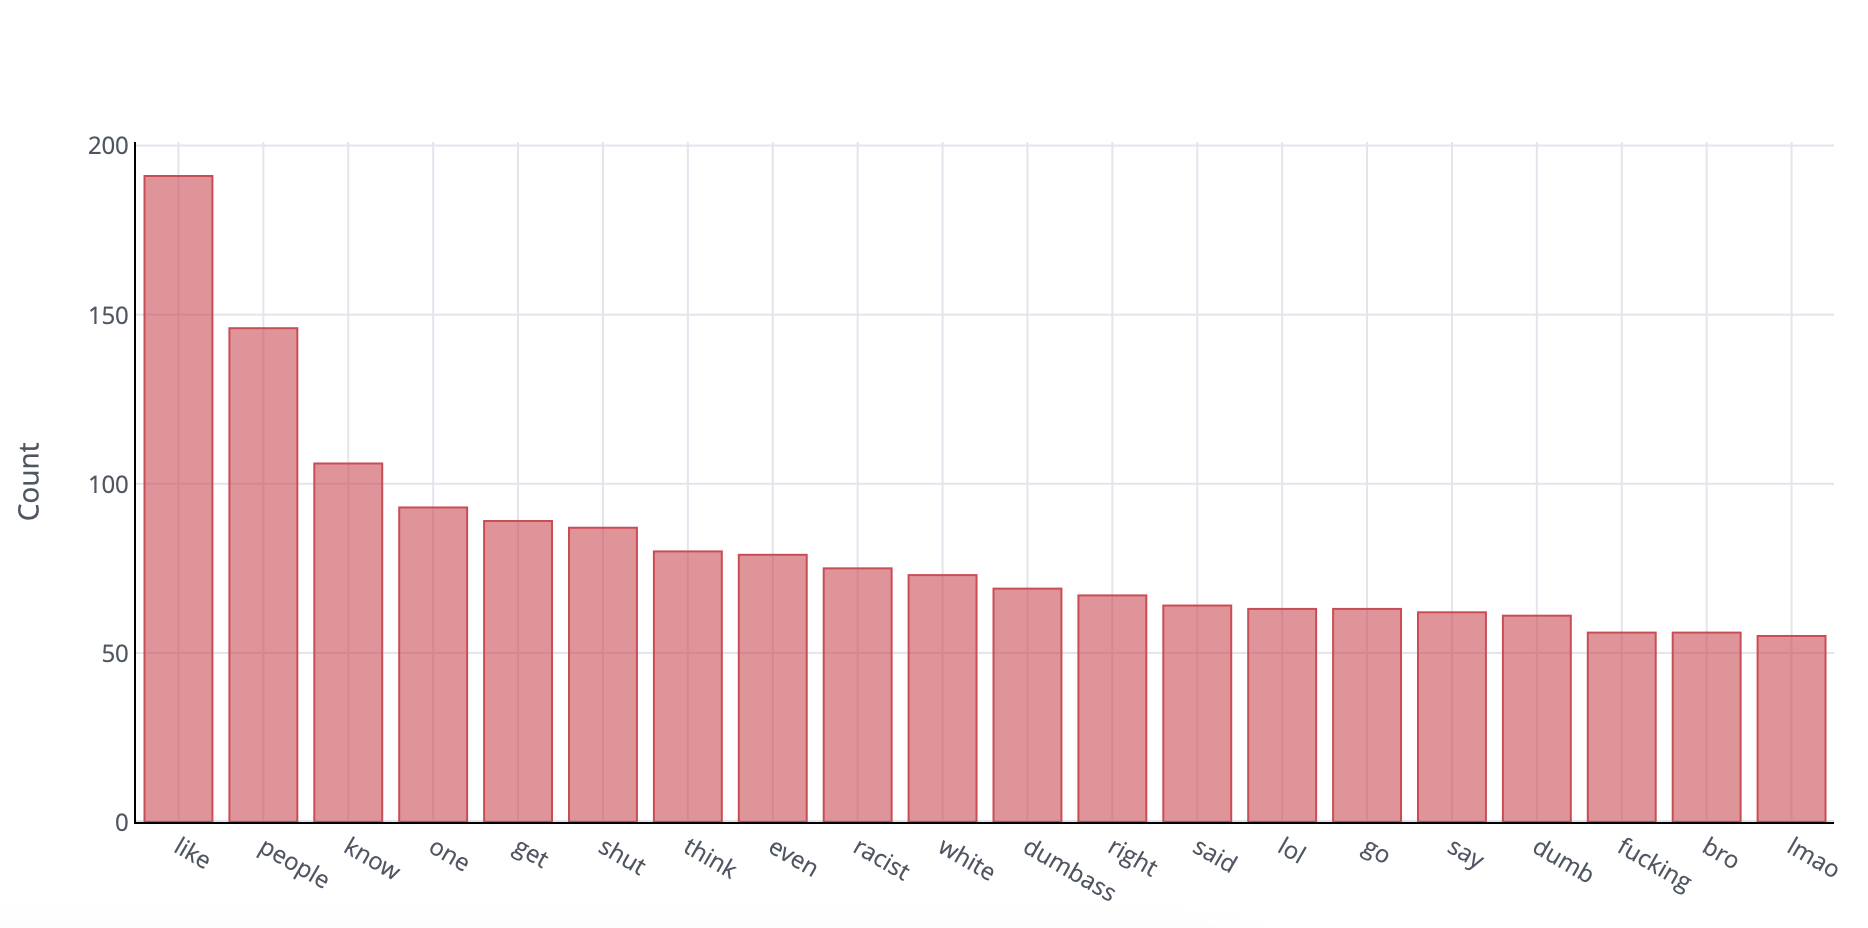}
		\caption{Top 20 words used for offensive comments after removing stop words}
		\label{fig:top20-after-removing-stopwords}
\end{figure}
\begin{figure}[h]
\centering
		\includegraphics[scale=0.33]{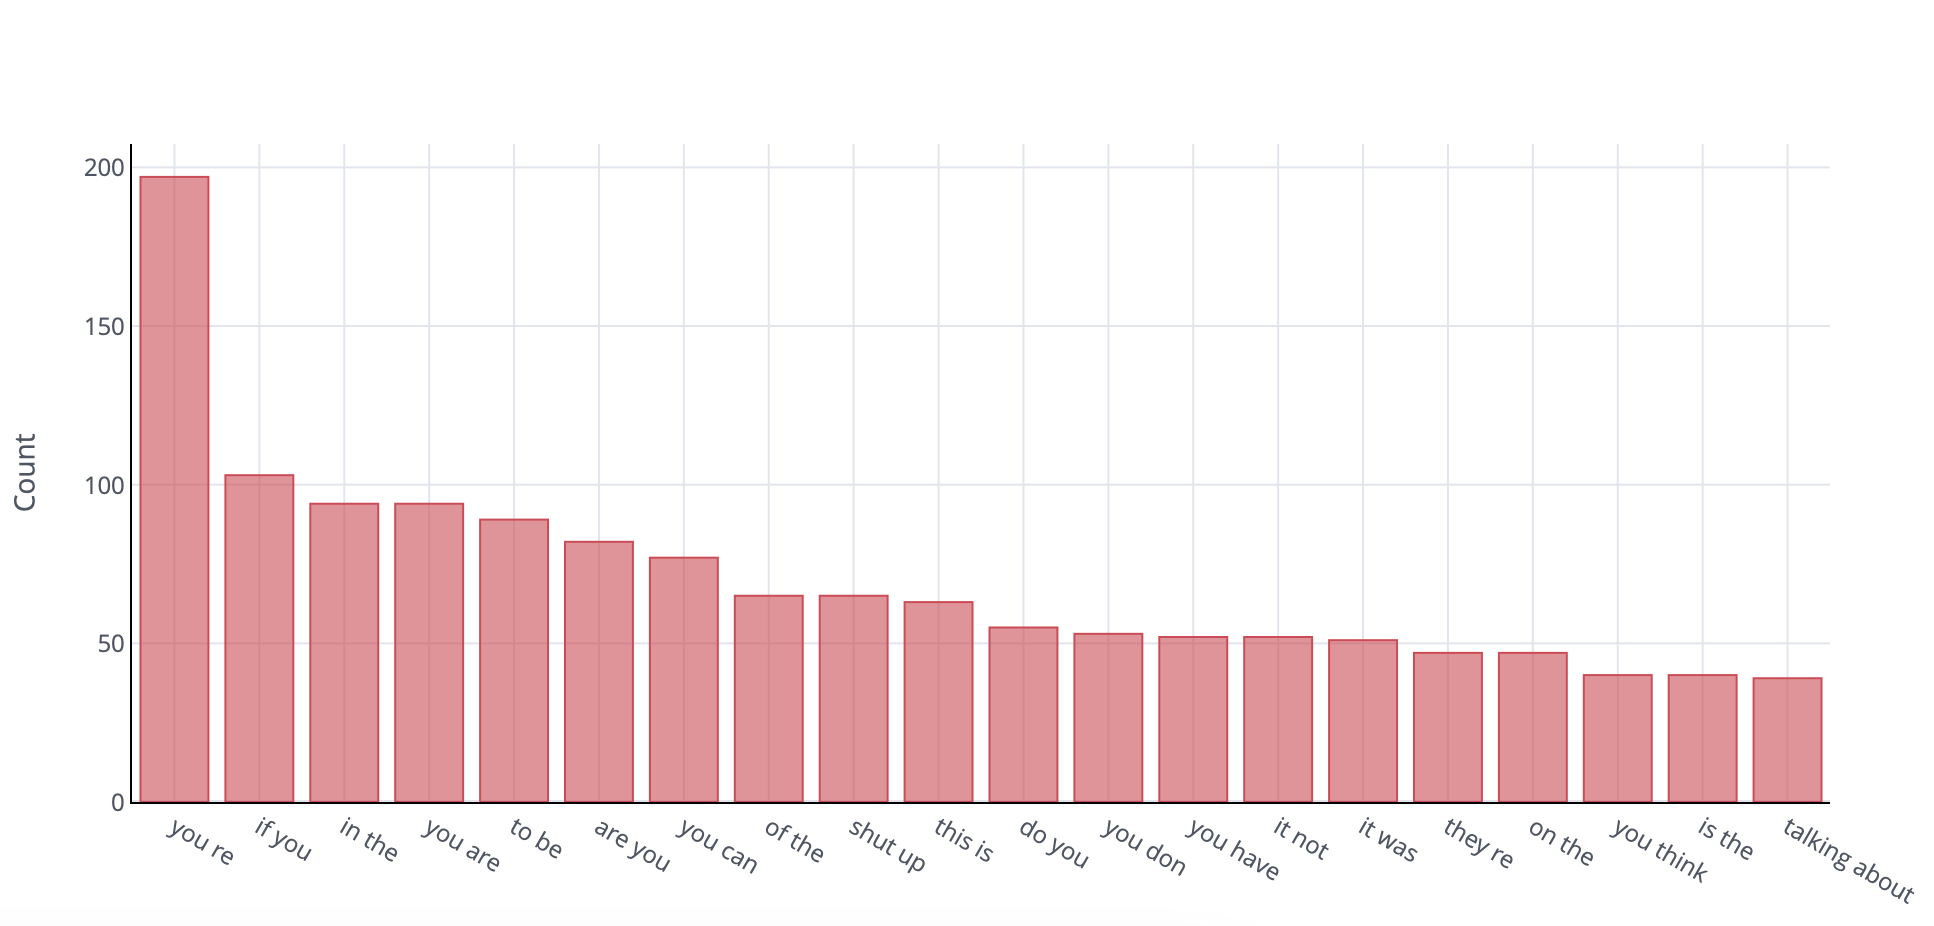}
		\caption{Top 20 bi-grams in offensive comments before removing stop words}
		\label{fig:top20-bigrams-before-removing-stopwords}
\end{figure}
\begin{figure}[h]
\centering
  		\includegraphics[scale=0.33]{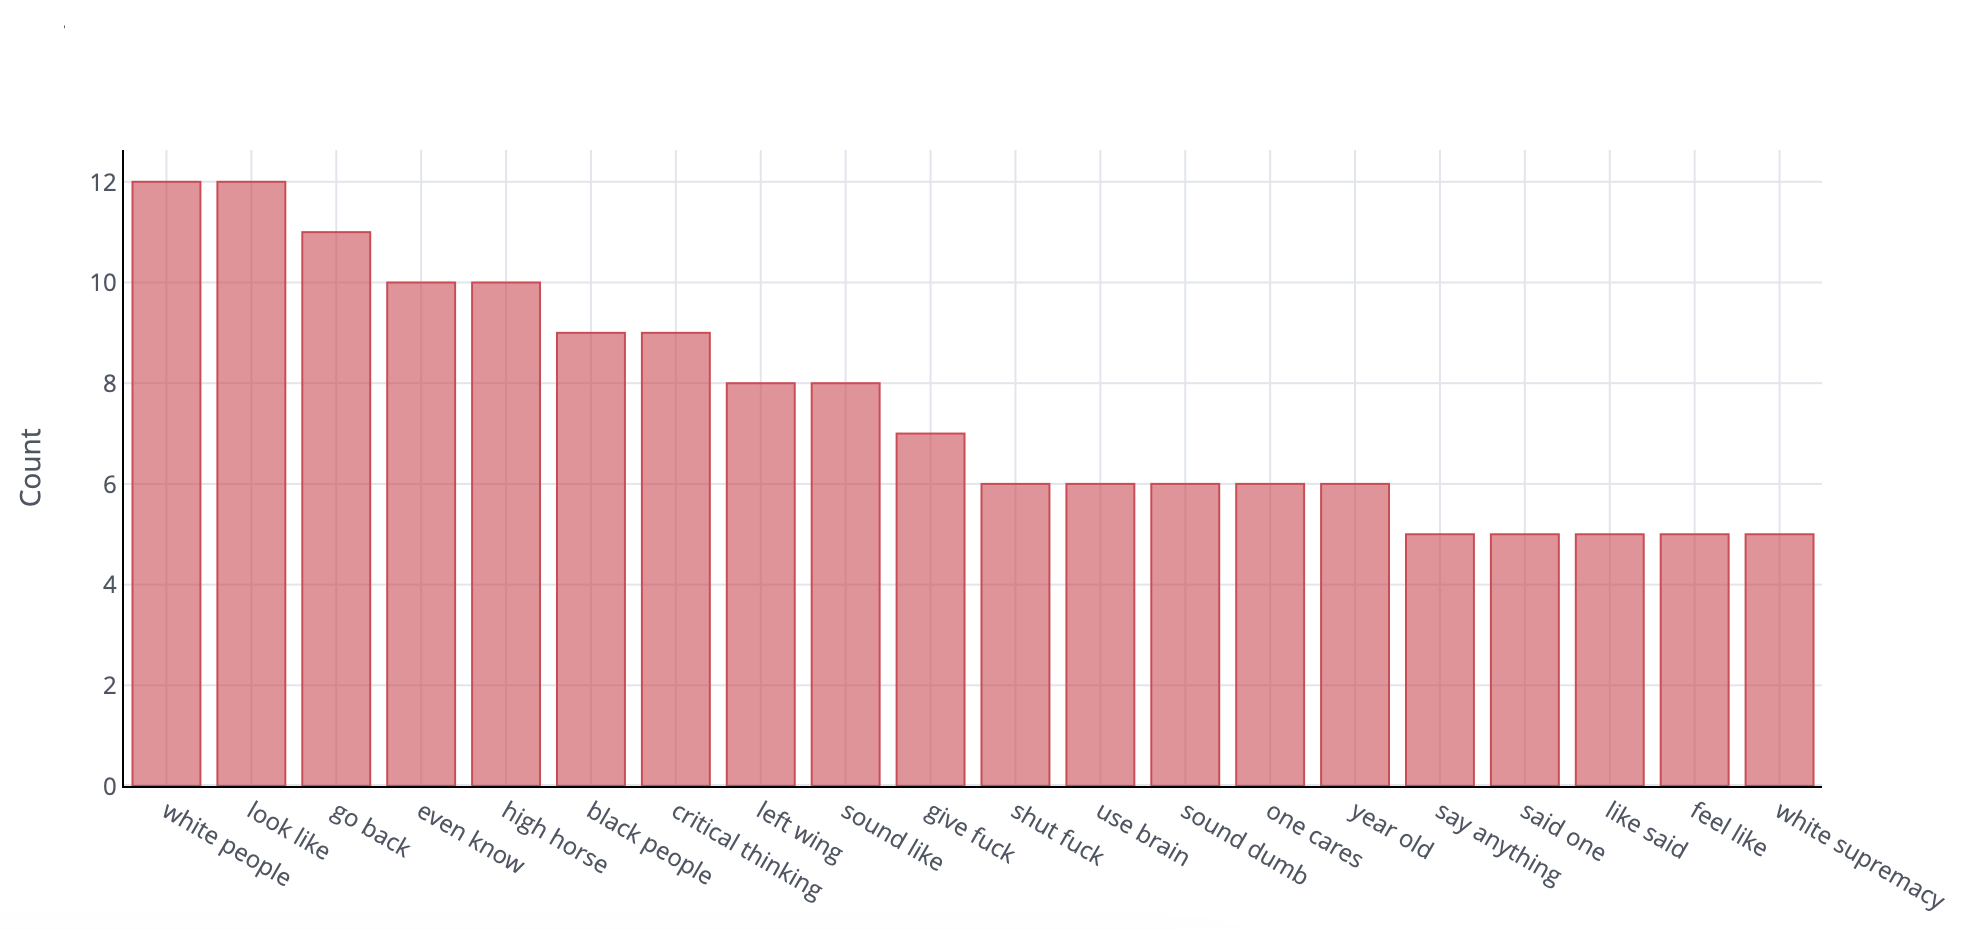}
		\caption{Top 20 bi-grams in offensive comments after removing stop words}
		\label{fig:top20-bigrams-after-removing-stopwords}
\end{figure}
\begin{figure}[h]
\centering
		\includegraphics[scale=0.33]{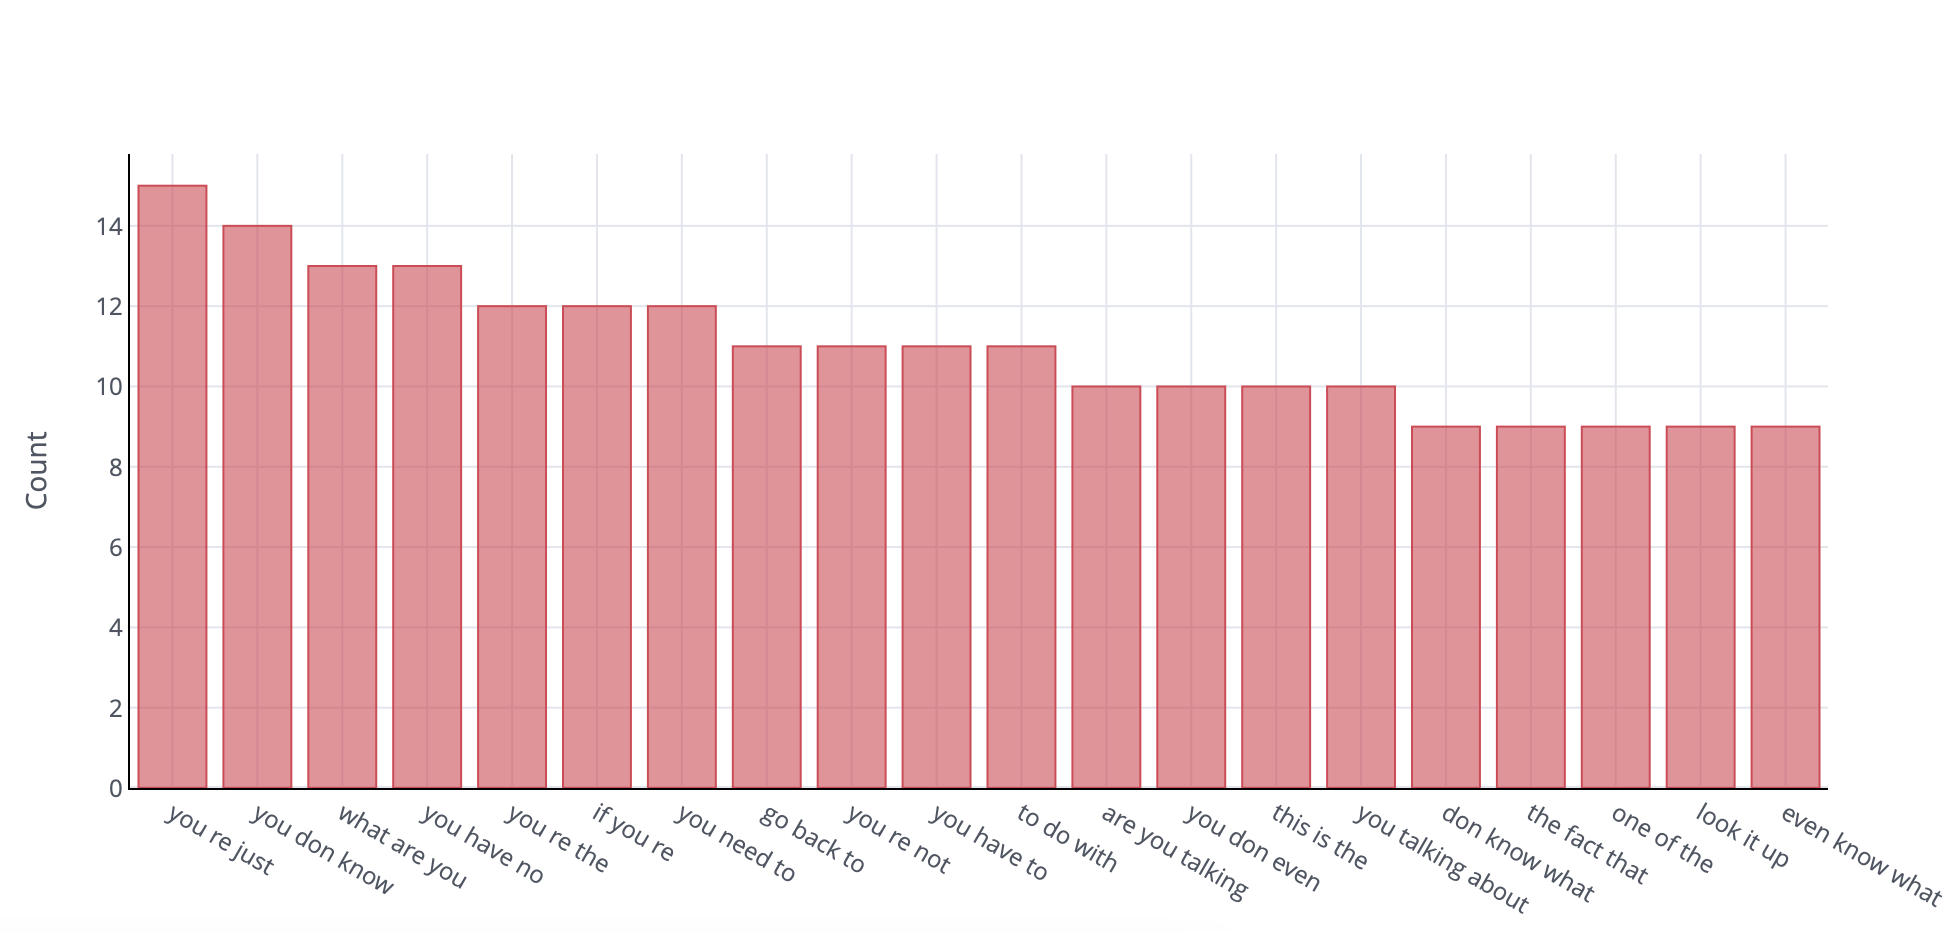}
		\caption{Top 20 tri-grams in offensive comments before removing stop words}
		\label{fig:top20-trigrams-before-removing-stopwords}
\end{figure}
\begin{figure}[h]
\centering
		\includegraphics[scale=0.33]{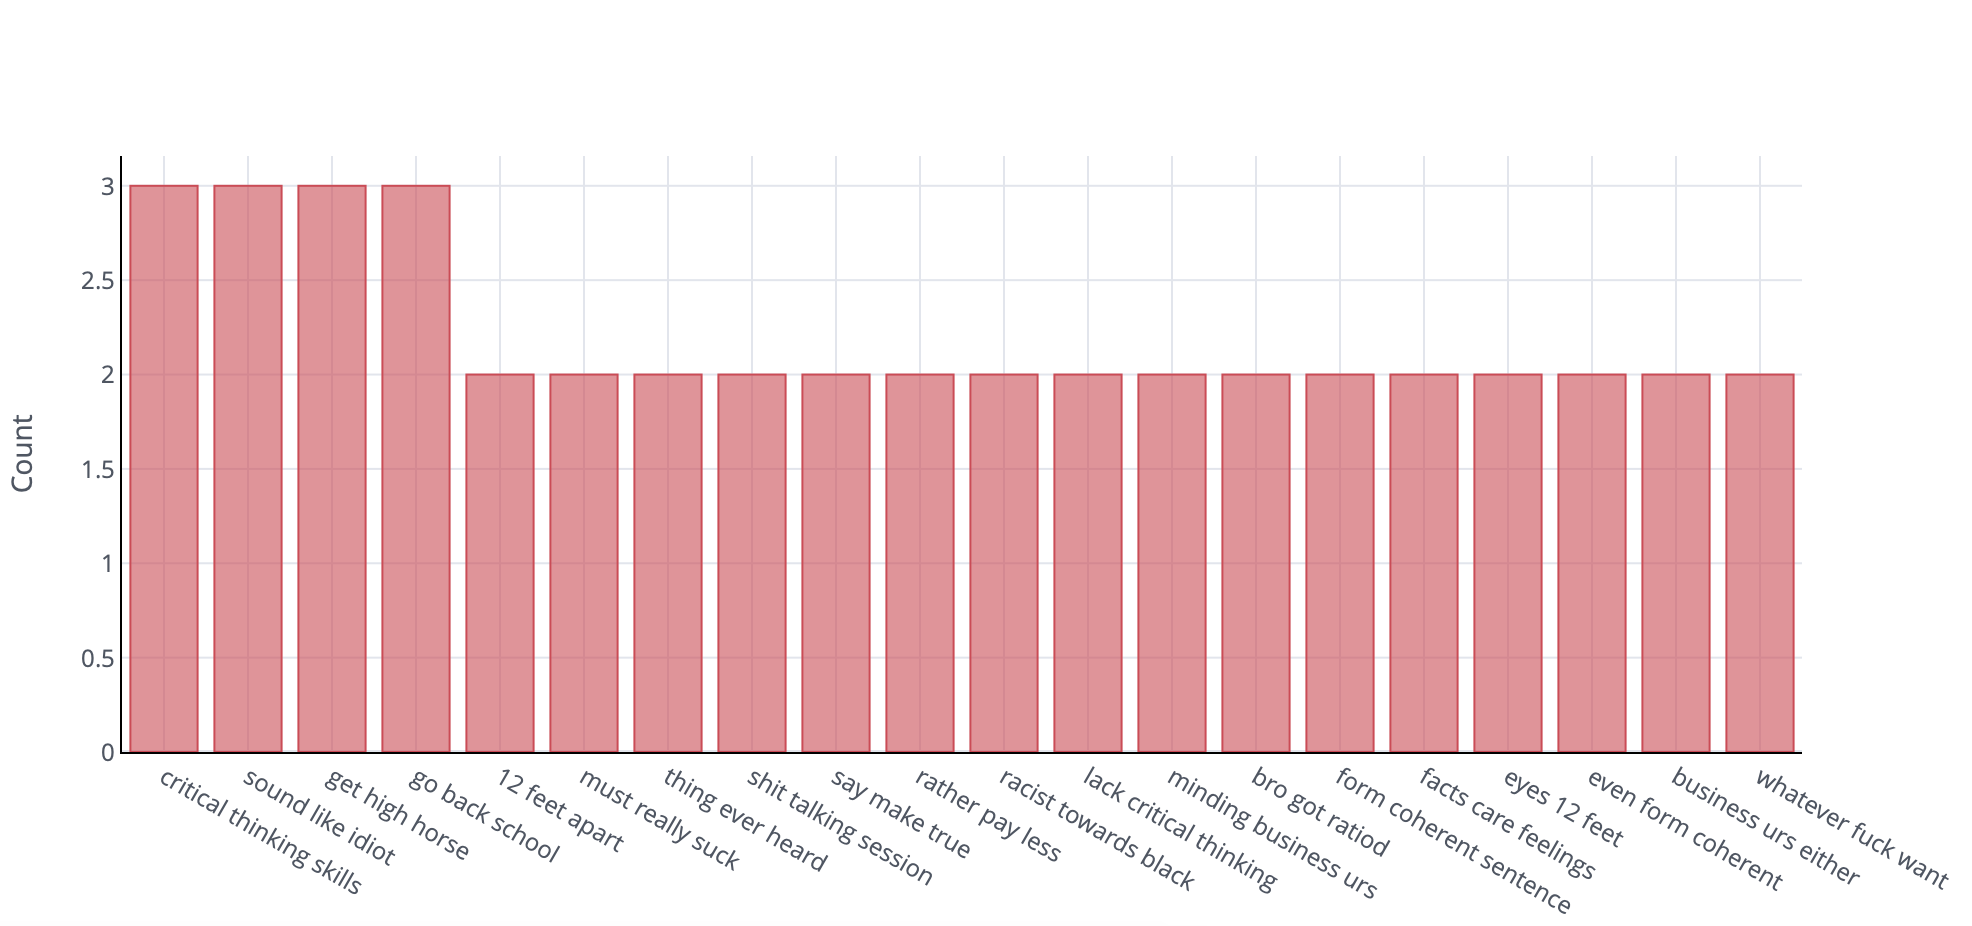}
		\caption{Top 20 tri-grams in offensive comments after removing stop words}
		\label{fig:top20-trigrams-after-removing-stopwords}
\end{figure}
